# Supplementary material for: Stacking-engineered ferroelectricity and multiferroic order in van der Waals magnets
Source: arXiv:2405.20069 source file (2025-01-09)
Supplement: Supplementary file 1 [file SM.pdf]

# SUPPLEMENTARY MATERIAL
# Stacking-engineered ferroelectricty and multiferroic order in van der Waals magnets

Daniel Bennett,[1,*] Gabriel Martínez-Carracedo,[2,3] Xu He,[4] Jaime Ferrer,[2,3] Philippe Ghosez,[4] Riccardo Comin,[5] and Efthimios Kaxiras[1,6]

[1] *John A. Paulson School of Engineering and Applied Sciences, Harvard University, Cambridge, Massachusetts 02138, USA*
[2] *Departamento de Física, Universidad de Oviedo, 33007 Oviedo, Spain*
[3] *Centro de Investigación en Nanomateriales y Nanotecnología, Universidad de Oviedo-CSIC, 33940 El Entrego, Spain*
[4] *Theoretical Materials Physics, Q-MAT, University of Liège, B-4000 Sart Tilman, Belgium*
[5] *Department of Physics, Massachusetts Institute of Technology, Cambridge, MA, USA*
[6] *Department of Physics, Harvard University, Cambridge, Massachusetts 02138, USA*

## FIRST-PRINCIPLES CALCULATIONS

First-principles density functional theory (DFT) calculations were performed using the SIESTA [1] code, version 5.0, with norm-conserving [2] PSML pseudopotentials [3], obtained from Pseudo-Dojo [4]. A basis of triple-$\zeta$ double polarized (TZDP) orbitals were used for all calculations, the cutoff radii of which were determined with an energy shift of 20 meV. Diffuse orbitals [5] were added ($5s$ and $5p$ for Ni, $6s$ and $6p$ for I) in order to better treat the interlayer interactions and the decay of the charge density into the vacuum region. We employed cutoff radii of 15 bohr for all diffuse orbitals, which were found to yield electronic band structures in good agreement with results obtained from the ABINIT plane-wave code [6] using the same PSML pseudopotentials. A Monkhorst-Pack $\mathbf{k}$-point grid [7] of $18 \times 18$ was used in all calculations and, the real space grid was determined with an energy cutoff of 1000 Ry. We use the PBE exchange-correlation functional [8] in all calculations. A DFT-D3 dispersion correction [9] was included in order to treat the long range interactions between the layers, with a dipole correction in the vacuum region to prevent dipole-dipole interactions between periodic images [10].

A Hubbard-$U$ correction was included on the Ni $3d$ orbitals with a value of $U = 1.8$ eV, following Ref. [11], where the value of $U$ and its effect on the magnetic ordering in nickel halide layers was carefully tested: it was found that the magnetic exchange parameters are qualitatively unaffected by the value of $U$ in the range 1–3 eV. SOC was included in all calculations except for geometry relaxation of the interlayer separation in the bilayers. The initial spin configuration was taken to be $\pm 2\mu_\mathrm{B}$ in the out-of-plane direction on the Ni atoms of each layer, the opposite (same) sign for AFM (FM) interlayer spin configurations. The spins did not deviate much from the initial configuration after convergence of the calculations, except for a small transfer of some spin to the I atoms.

A lattice constant of 4.00 Å was obtained for monolayer $NiI_2$, in good agreement with the experimentally reported value of 3.98 Å, which was used in the bilayer calculations. Geometry relaxations were then performed (without SOC) in order to determine the interlayer separation, using a force tolerance of 0.1 meV/Å. The top layer was translated above the bottom layer along the unit cell diagonal, for both aligned and anti-aligned stacking configurations, and for both AFM and FM interlayer spin configurations. After relaxation, calculations were then repeated including SOC. The polarization was calculated from Berry phases.

Because the volume, and hence the polarization, is ill-defined in 2D materials, we plot the dipole moment in the main text. In order to better compare with conventional ferroelectrics, we plot the stacking-dependent polarization in Fig. S1. Here, the volume of the bilayer is defined to be the in-plane area of the unit cell times the interlayer separation, which is taken to be the vertical separation between the Ni atoms in each layer.

* dbennett@seas.harvard.edu

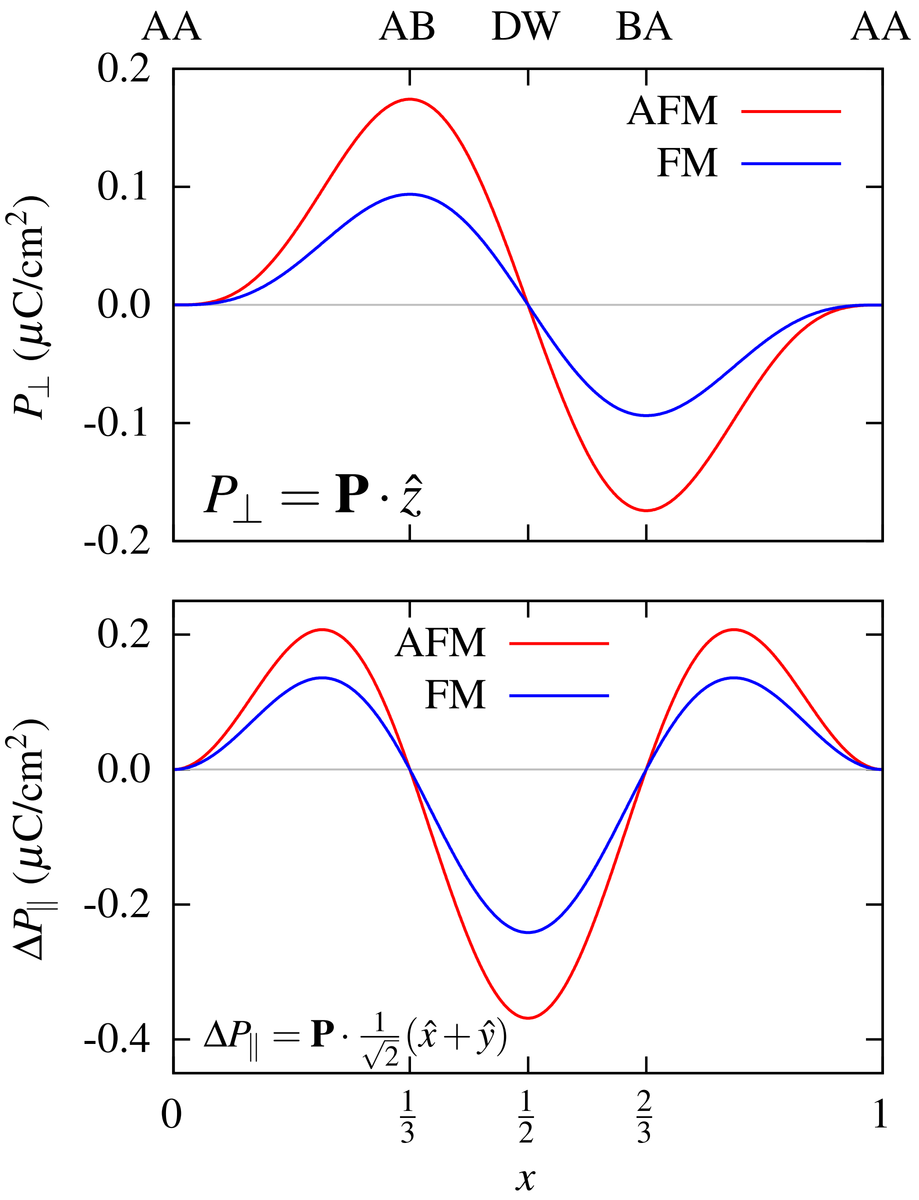


FIG. S1. Plot of the out-of-plane (top) and in-plane (bottom) polarization as a function of stacking in anti-aligned bilayer $NiI_2$, for AFM (red) and FM (blue) interlayer spin configurations.

**DIFFERENTIAL CHARGE DENSITY**

Fig. S2 shows the differential electronic charge density of anti-aligned $NiI_2$ for the AB and BA stackings, obtained using the C2X utility [12]. We can see that the direction of the transferred charge switches upon changing the stacking configurations. Upon changing the interlayer spin order, a small difference in the differential charge density is observed.

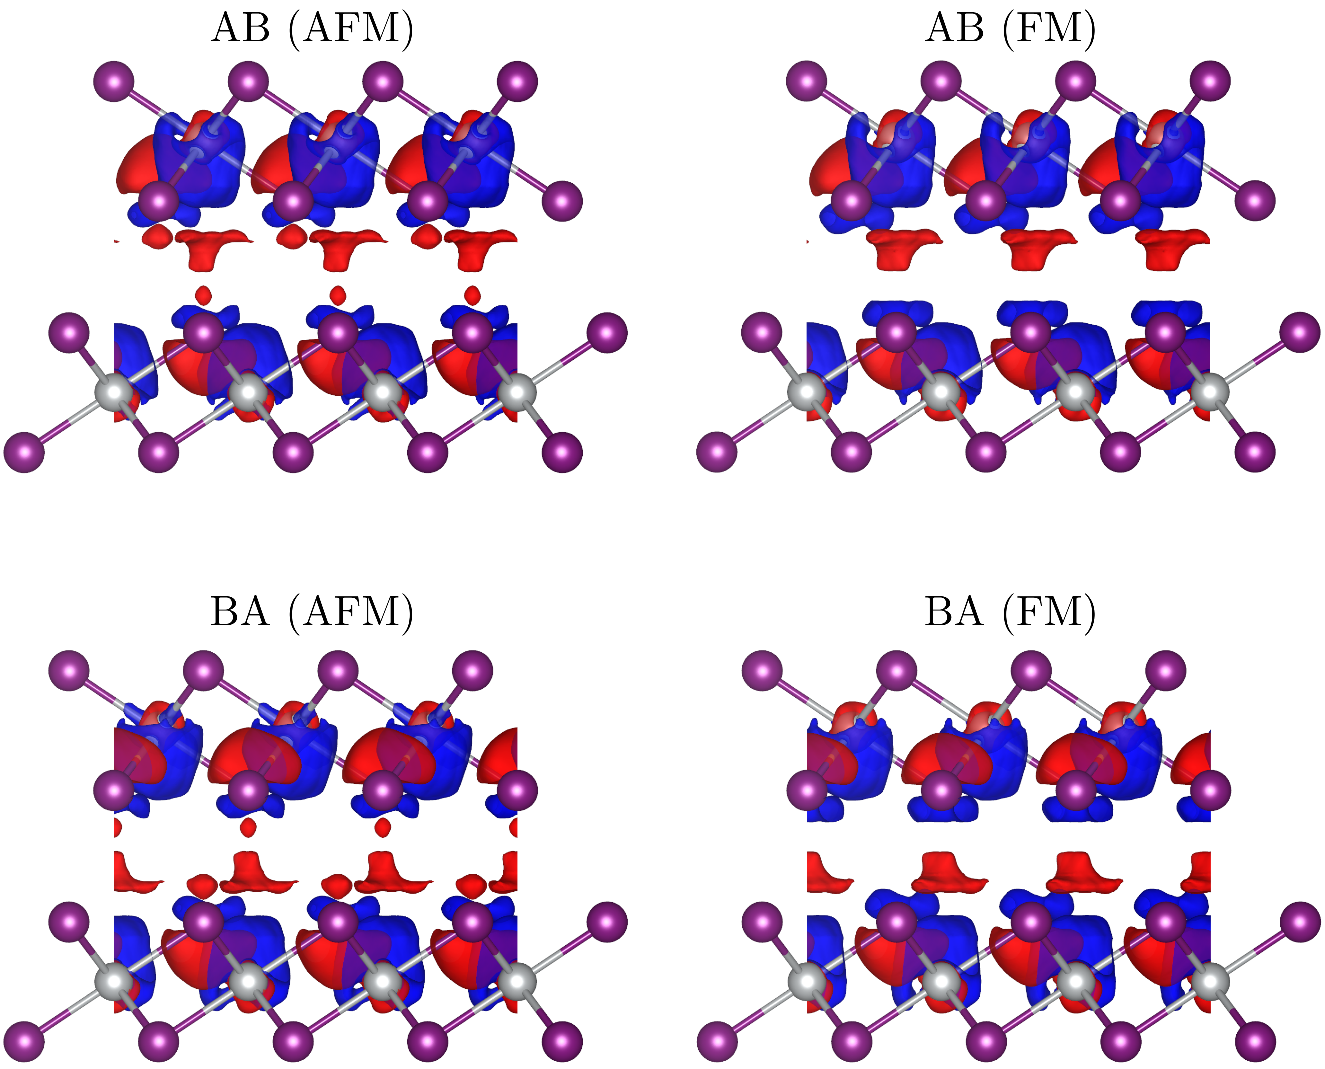


FIG. S2. Differential charge densities for the AB/BA stackings and AFM/FM interlayer spin configurations, obtained by subtracting the total real-space charge densities of the individual monolayers from the total density of the bilayer in each case. The blue and red isosurfaces correspond to negative and positive charge, respectively.

## ORBITAL-PROJECTED BAND STRUCTURES

Fig. S3 shows the orbital-projected electronic band structures of AB stacked anti-aligned $NiI_2$ for the AFM and FM interlayer spin configurations. The valence bands and top two conduction bands mainly consist of strong hybridization between the Ni 3$d$ states and the I 5$p$ states, and the higher conduction bands are mainly described by the Ni 4$s$ states. Changing from the AFM to the FM spin order results in small splittings in the bands due to the breaking of time reversal symmetry. Although the general orbital character of the bands remains the same upon changing the spin order, these small changes in the electronic structure result in a change in electronic polarization. While the changes are small, the electronic charge transfer is weak, and small changes in the electronic structure are sufficient to cause a large relative change in polarization, by a factor of $\sim 2$.

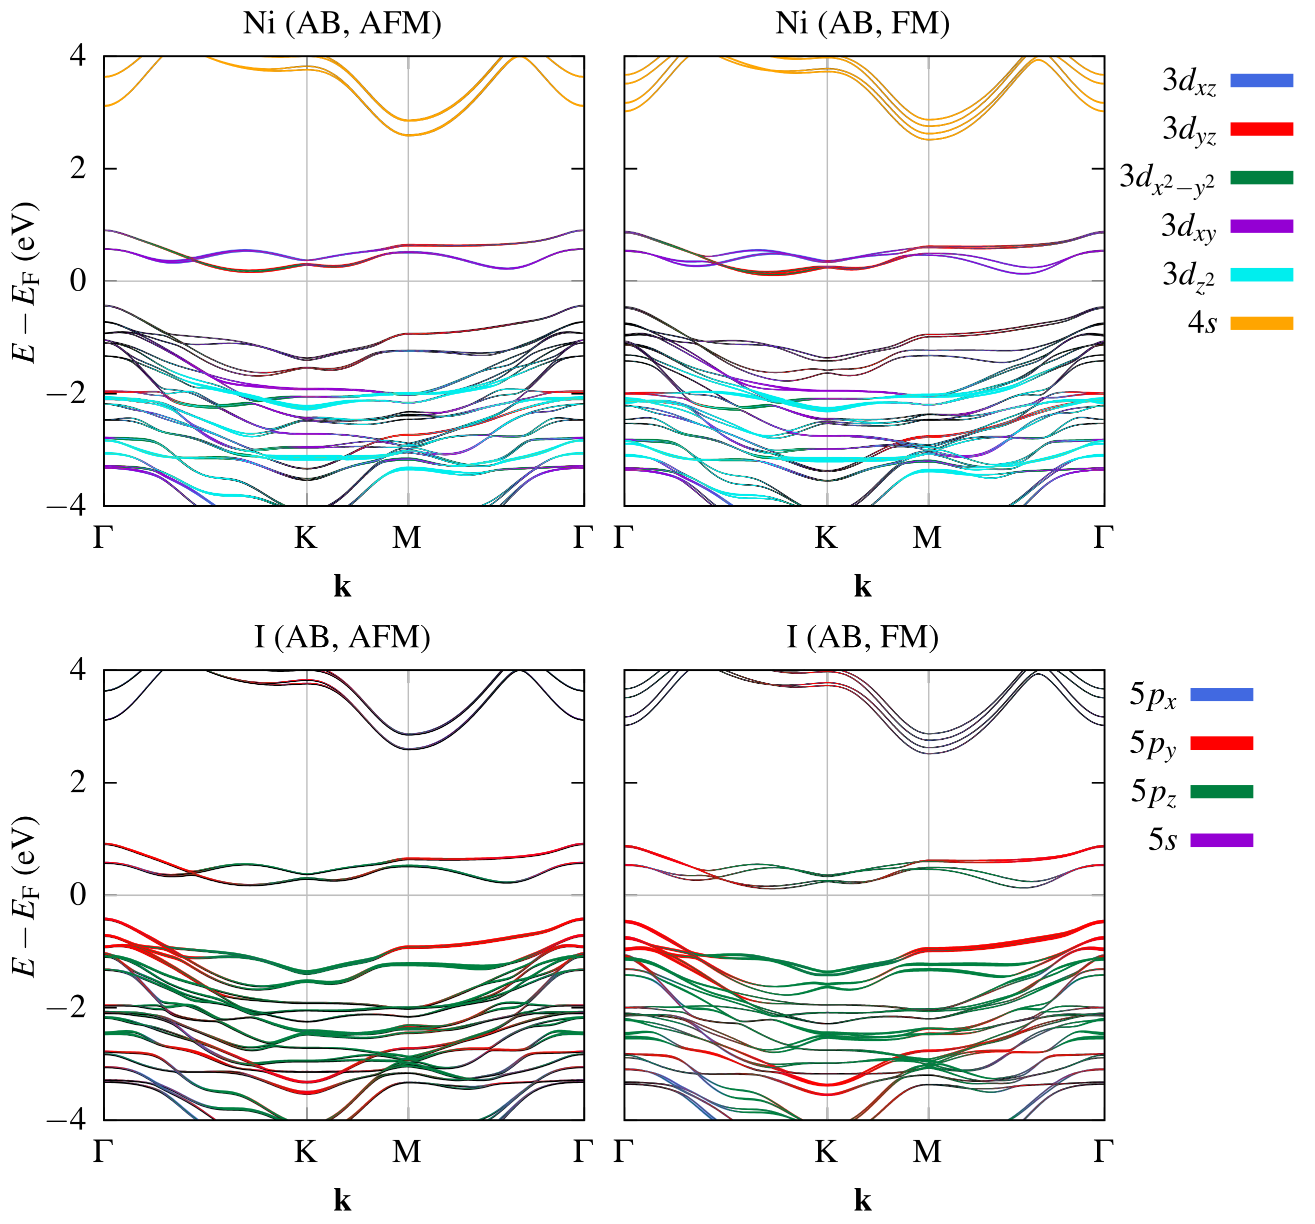


FIG. S3. Orbital-projected band structures for anti-aligned bilayer NiI2 for the AB stacking, and for AFM (left) and FM (right) interlayer spin configurations. Projections onto Ni (top) and I (bottom) orbitals are shown separately.

## TOPOLOGICAL POLARIZATION

The total polarization, including both in-plane and out-of-plane components and the winding of the polarization are shown as a function of stacking in Fig. S4 for AFM and FM anti-aligned bilayer $NiI_2$.

The winding of the polarization field (topological charge) was calculated following the methodology in Ref. [13]. The total winding number is given by

$$Q = \frac{1}{4\pi}\int \mathbf{P}\cdot(\partial_x\mathbf{P}\times\partial_y\mathbf{P})\,\mathrm{d}\mathbf{x}\,, \tag{S1}$$

where $\mathbf{P}$ is normalized and $\mathbf{x}=(x,y)$. The polarization in the unit cell is discretized on a fine grid with spacing $\Delta$, and a plaquette is constructed around each grid point. The plaquettes form a grid which is offset from the original by half a grid spacing, which avoids the nonpolar AA stacking. The local winding or topological charge can then be defined as

$$q(\mathbf{x}) = \frac{1}{4\pi}\left(A(P_1,P_2,P_3)+A(P_1,P_3,P_4)\right)\,, \tag{S2}$$

where $A$ is the signed area spanned by three points on a sphere:

$$\begin{aligned}A(P_1,P_2,P_3) = 2\arg\big(&1+P_1\cdot P_2+P_2\cdot P_3+P_3\cdot P_1\\ &+iP_1\cdot(P_2\times P_3)\big)\end{aligned}\,. \tag{S3}$$

$q(\mathbf{x})$ is shown in Figs. S4 (c) and (f) for AFM and FM anti-aligned bilayer $NiI_2$, respectively. The total charge is then given by

$$Q = \sum_{\mathbf{x}} q(\mathbf{x})\,. \tag{S4}$$

The winding numbers of AB and BA domains converge to $Q_{\mathrm{AB}} = -Q_{\mathrm{BA}} = \frac{1}{2}$ with grid spacing $\Delta$.

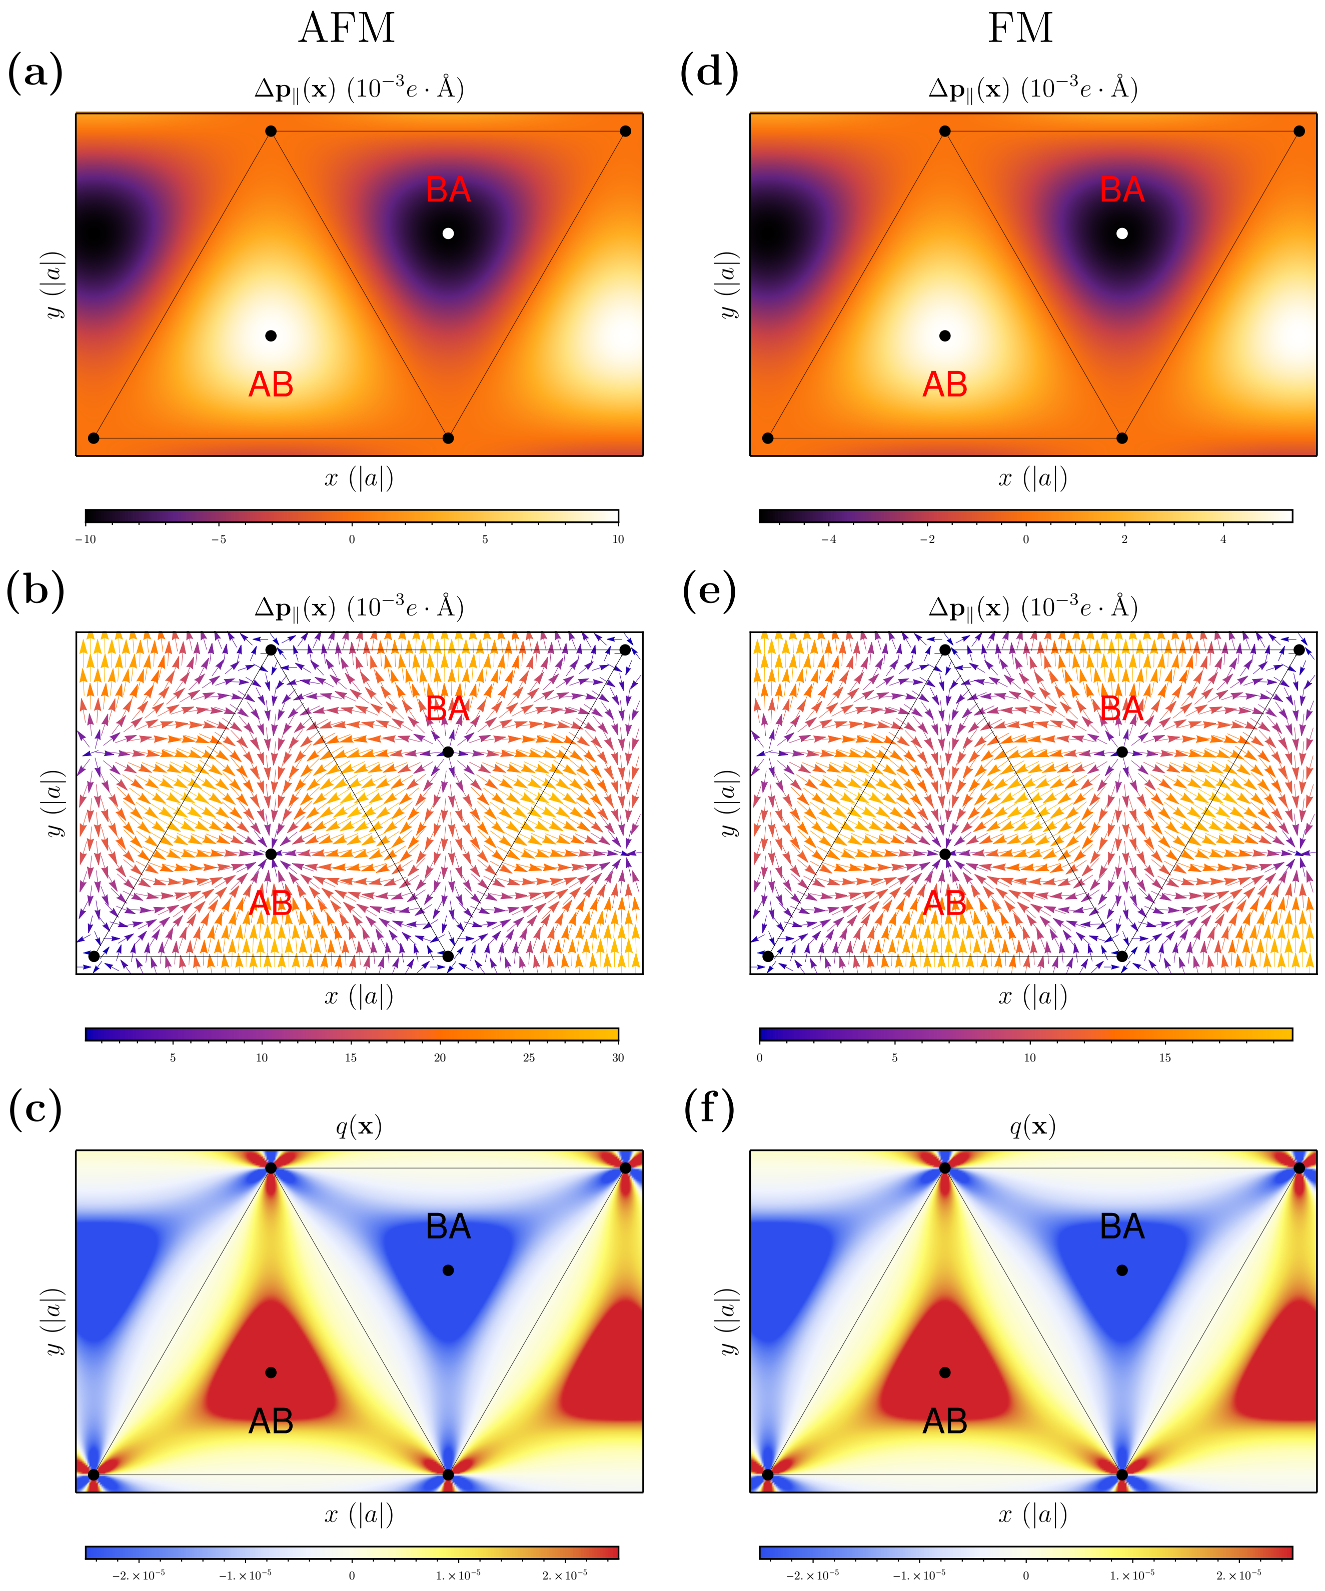


FIG. S4. **(a)**–**(c)** Polarization in the **(a)** out-of-plane and **(b)** in-plane directions, and **(c)** winding of the total polarization, as a function of relative stacking in AFM anti-aligned bilayer $NiI_2$. **(d)**–**(f)** Polarization in the **(d)** out-of-plane and **(e)** in-plane directions, and **(f)** winding of the total polarization, as a function of relative stacking in FM anti-aligned bilayer $NiI_2$.

## MAGNETIC EXCHANGE PARAMETERS

The GROGU code [14] was used to calculate the intralayer magnetic exchange parameters of the Heisenberg Hamiltonian in Eq. 3 in the main text. As the dominant DM interaction is given by first nearest neighbors and the radial component is negligible, it is convenient to express DM vectors in cylindrical coordinates $\mathbf{D}^{ij} = (D^r, D^\theta, D^z)$ where the radial component points along the bond.

GROGU calculations were performed using a dense Monkhorst-Pack grid of $100 \times 100$ which take a self-consistent Hamiltonian obtained from SIESTA calculations (including SOC). The localized magnetic entities were projected onto $3d$-orbitals of the Ni atoms.

Fig. S5 shows the exchange parameters between the Ni atoms in bilayer $NiI_2$ as a function of stacking. The intralayer parameters $J_\parallel$ were calculated using the LKAG method [15], which are slightly modulated as a function of stacking. The interlayer exchange parameters $J_\perp$ are governed by long-range electrostatic interactions, meaning that they are very sensitive to many computational parameters. We therefore estimate them from the total energy differences between the AFM and FM interlayer spin configurations at each stacking. A more detailed treatment of the interlayer exchange interactions in vdW magnets using the LKAG method is left for a subject of future research. The nearest neighbor (NN) intralayer interactions are underestimated when compared to the value obtained in Ref. [11], which uses the supercell method. This is due to the strong hybridization between the Ni and I atoms in each layer, which carry much of the exchange. However, the LKAG method allows us to calculate exchanges between an arbitrary number of NNs using a single unit cell, and study the stacking dependence of the magnetic properties. The interlayer exchange changes by as much as a factor of 2 as a function of stacking. The interlayer spin order however, does not change upon changing the stacking, in contrast to e.g. $CrI_3$ [16], and the AFM spin order is always energetically preferable at zero electric field. Because inversion symmetry is broken, the DM vectors are non-zero in the bilayer.

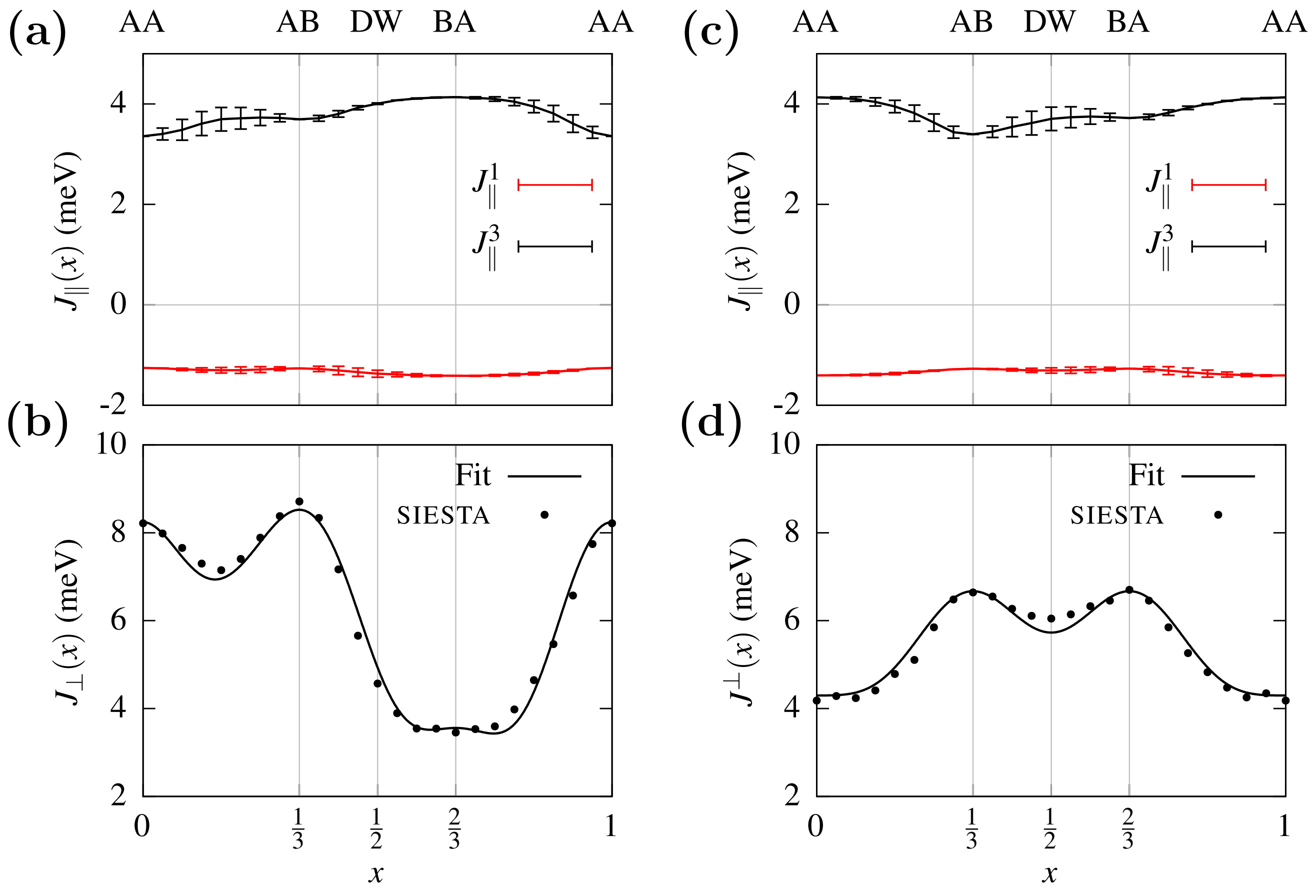


FIG. S5. Intralayer $J_\parallel$ and interlayer $J_\perp$ exchange as a function of stacking for **(a)**,**(b)** aligned and **(c)**,**(d)** anti-aligned bilayer $NiI_2$. In **(a)** and **(c)**, mean averages over the first ($J_\parallel^1$) and third nearest neighbors ($J_\parallel^3$) are shown, where the error bars indicate the corresponding mean square deviation. The points in **(b)** and **(d)** show the total energy differences from DFT calculations, the solid line was obtained using the fits to the stacking energy in Fig. 1 in the main text.

Fig. S6 shows the mean values of $\theta$ and $z$ DM components in cylindrical coordinates for the first shell of NN atoms. These mean magnitudes reach values as large as 0.1 meV, corresponding to about $\sim 10\%$ of $J^1_{\parallel}$, which may alter the behavior of the different spin textures in the bilayer. We note that the angular component $D^\theta$ changes sign in the FM configurations as a function of stacking as shown in Figs. S6 (b) and (d). This conveys a change in the in-plane chirality of the DM vector, where $D^\theta > 0$ and $D^\theta < 0$ imply right- and left-handed chirality, respectively.

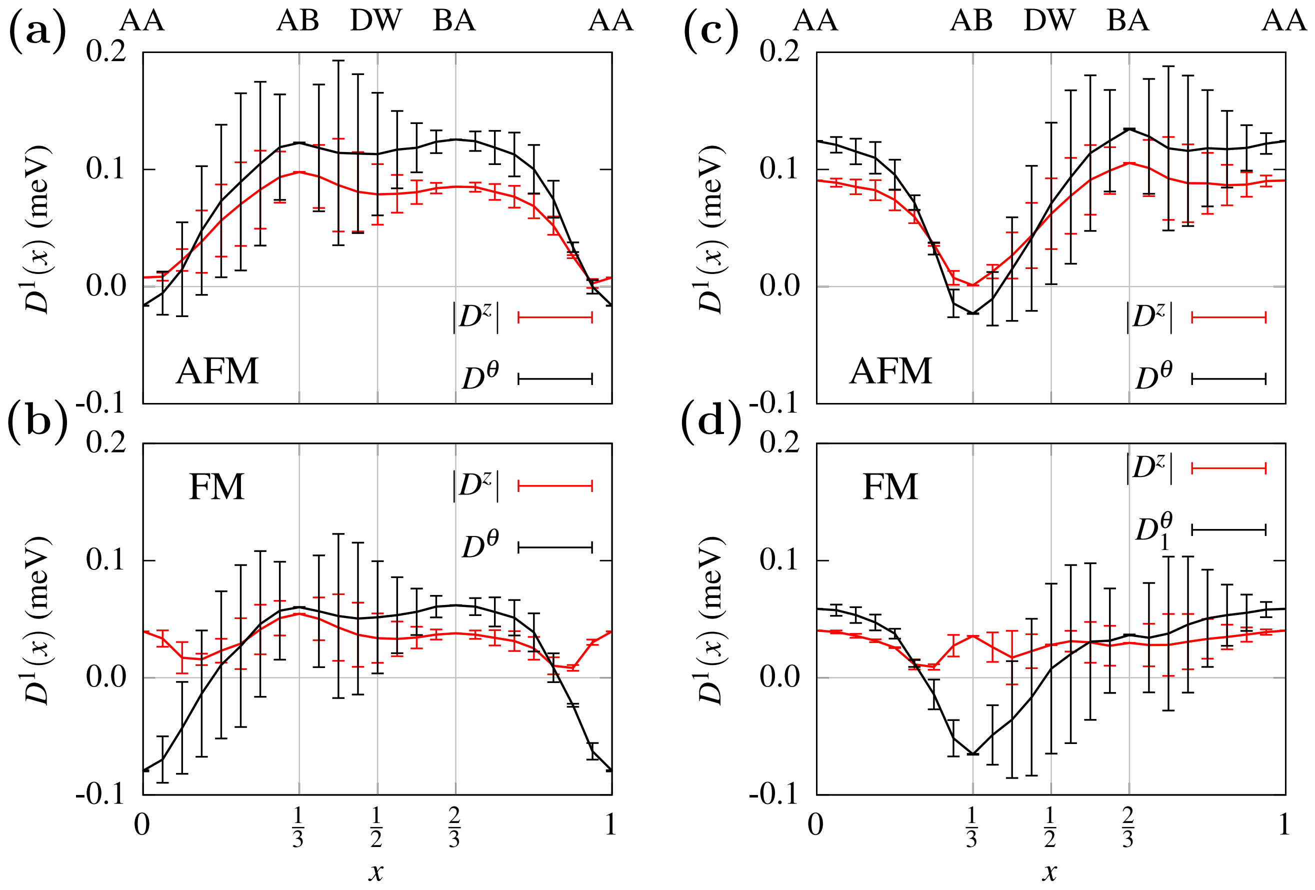


FIG. S6. Angular ($\theta$) and $z$ components of the first-neighbor DM vectors, averaged over the six neighbors for **(a)**,**(b)** aligned and **(c)**,**(d)** anti-aligned bilayer $NiI_2$. Choosing a cylindrical coordinate system where the radial component is oriented along each respective bond is more convenient because the radial components are all negligible, meaning that only the angular $D^\theta$ components need to be considered. The error bars show the mean square deviations. Note that $D^\theta$ and $D^z$ respond differently to the change in relative stacking.

The intralayer magnetic exchange parameters for individual NNs are shown in Fig. S7, for aligned and anti-aligned stackings, as well as AFM and FM interlayer spin configurations. The exchange is shown for the six 1st NNs, which are linear combinations of the lattice vectors: $\mathbf{v}_n^1 = i\mathbf{a}_1 + j\mathbf{a}_2$ such that $\left|\mathbf{v}_n^1\right| = 1$. The indices $(i,j)$ for $\mathbf{v}_n^1$ are, in order:

$$\mathbf{v}_1^1 = (0,1), \quad \mathbf{v}_2^1 = (1,0), \quad \mathbf{v}_3^1 = (-1,0), \quad \mathbf{v}_4^1 = (0,-1), \quad \mathbf{v}_5^1 = (1,-1), \quad \mathbf{v}_6^1 = (-1,1)\ . \tag{S5}$$

The exchange is also shown for the six 3rd NNs, where $\mathbf{v}_n^3 = 2\mathbf{v}_n^1$. There is a splitting between neighbors 1–4 and 5–6 as a function of relative stacking.

Fig. S8 shows the $D^\theta$ and $|D^z|$ components of the DM vector as a function of relative stacking, which also has a splitting between neighbors 1–4 and 5–6.

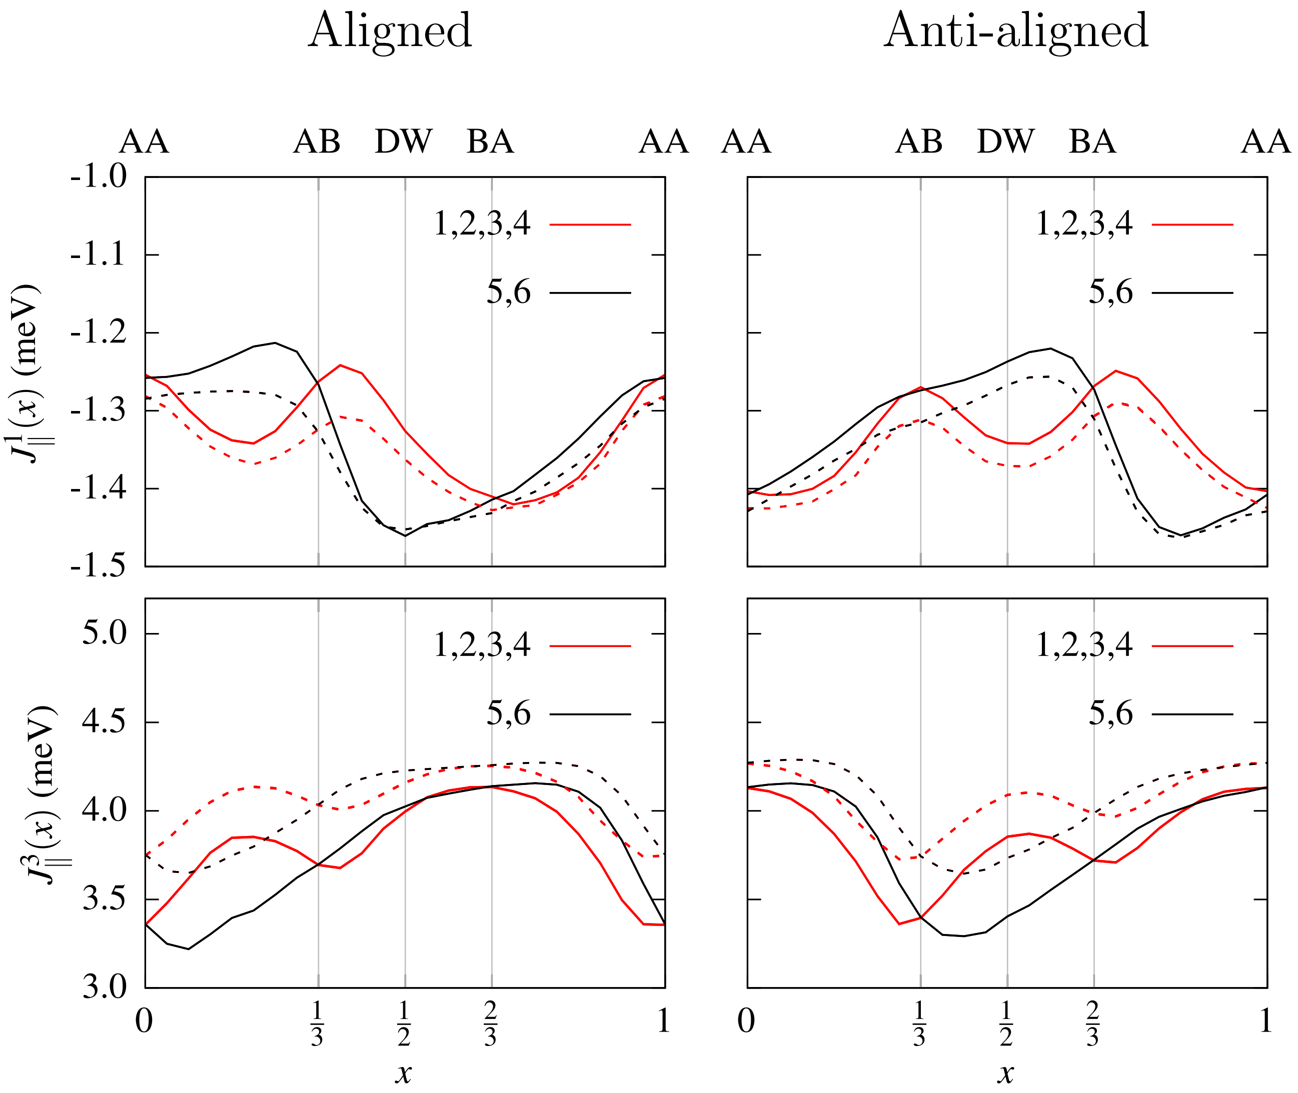


FIG. S7. 1st NN (top) and 3rd NN (bottom) intralayer exchange parameters as a function of relative stacking in aligned (left) and anti-aligned (right) bilayer $NiI_2$. The solid and dashed lines represent the AFM and FM interlayer spin order, respectively. Neighbors 1–4 are represented by the red lines, and neighbors 5–6 are represented by the black lines.

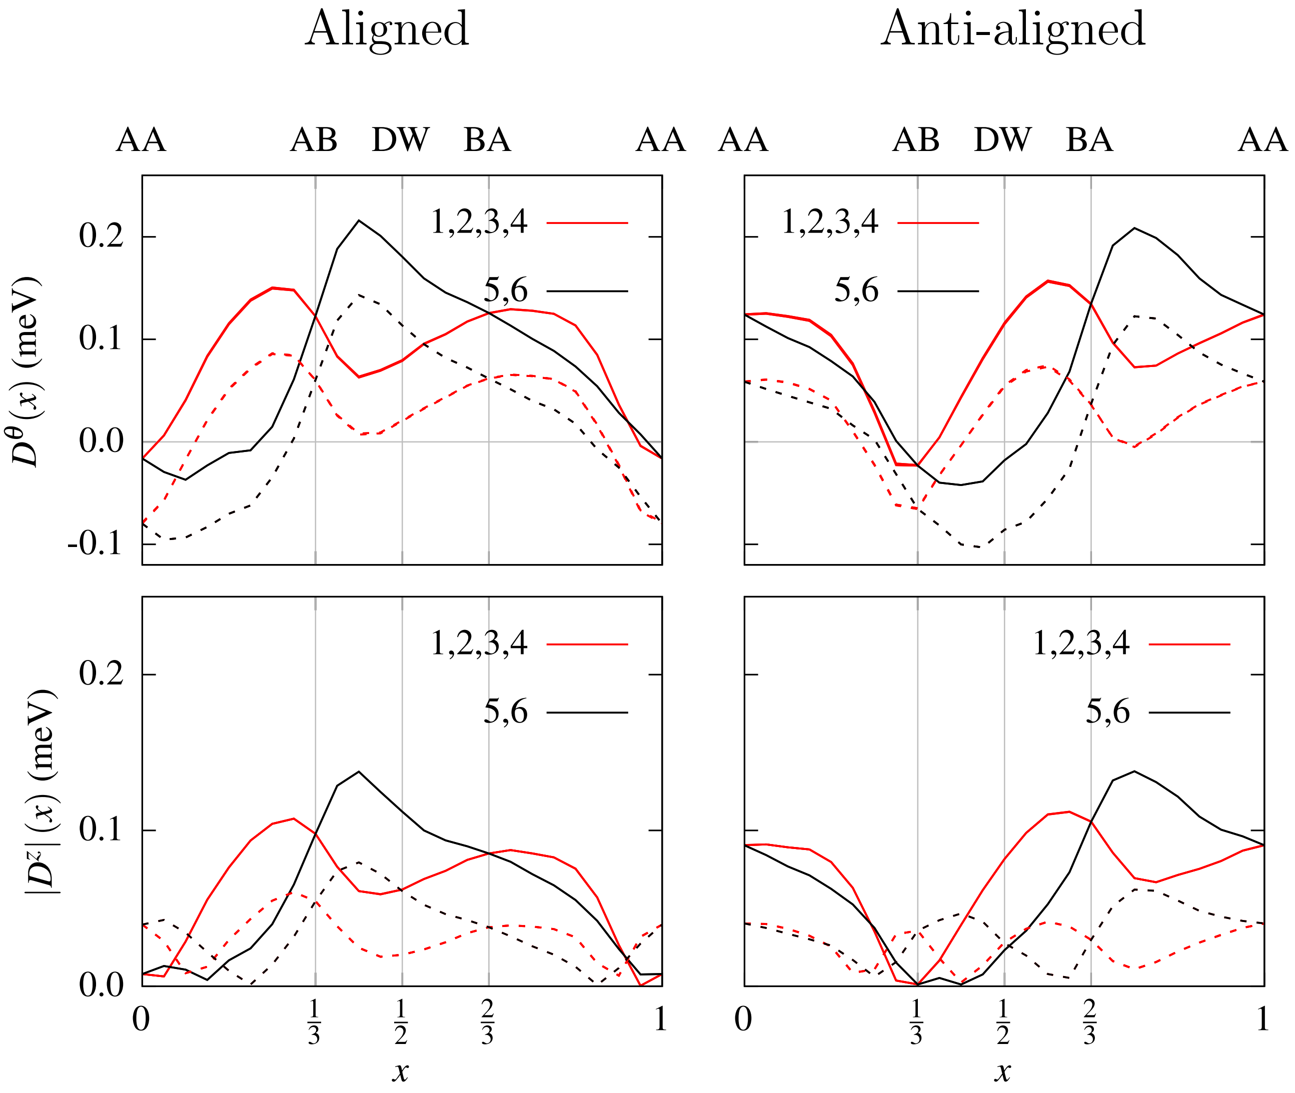


FIG. S8. $D^\theta$ (top) and $|D^z|$ (bottom) components of the DM vector as a function of relative stacking in aligned (left) and anti-aligned (right) bilayer $NiI_2$. The solid and dashed lines represent the AFM and FM interlayer spin order, respectively. Neighbors 1–4 are represented by the red lines, and neighbors 5–6 are represented by the black lines.

## MONTE CARLO SPIN SIMULATIONS

MC simulations were performed using the Heisenberg model:

$$H = H_{\text{intra}} + H_{\text{inter}} - \sum_i \mathbf{B} \cdot \mathbf{S}_i \,, \tag{S6}$$

where $H_{\text{intra}}$ and $H_{\text{inter}}$ are given by Eqs. 3 and 4 in the main text, and the last term is the Zeeman interaction. The intralayer exchange parameters for monolayer $NiI_2$ from Ref. [11] were used, which were calculated using the supercell method, because the exchange parameters calculated using the LKAG method underestimate the intralayer exchanges (1$^{\text{st}}$ NN in particular) due to the strong hybridization between the Ni and I atoms in each layer. The 1$^{\text{st}}$, 2$^{\text{nd}}$ and 3$^{\text{rd}}$ NN exchange parameters are $J_{\parallel}^{1} = -7.0$ meV, $J_{\parallel}^{2} = -0.3$ meV and $J_{\parallel}^{3} = +5.8$ meV, respectively. In addition, the anisotropic exchange parameters for the 1$^{\text{st}}$ NNs between Ni atoms are taken into account. For the interlayer interaction, we take only the NN exchange parameter, and estimate that with the energy difference between the ferromagnetic and antiferromagnetic interlayer alignments, which gives a $J_{\perp} = 7$ meV. Calculations were repeated using the exchange parameters obtained in this work. The results using both sets of exchange parameters are compared in SM.

We then perform Metropolis MC simulations to estimate the magnetic field required to align the interlayer magnetic moments. The calculations are performed using a $64 \times 64$ supercell, with periodic boundary conditions in the in-plane directions. Calculations were repeated using a $128 \times 128$ supercell to check the convergence with respect to system size, see Fig. S9. The results are virtually identical, suggesting that results are sufficiently converged for a $64 \times 64$. An additional calculation using a $1 \times 1$ cell was performed so that intralayer interaction is constrained to be FM. We note that if the intralayer spin is constrained to be FM, the coercive magnetic field is much smaller, approximately 25 T with an in-plane magnetic field, which is consistent with the estimation from firs-principles calculations, or approximately 120 T with an out-of-plane magnetic field.

Monte Carlo spin simulations were performed using both the exchange values obtained in Ref. [11], and this work, see Fig. S10. The 1$^{\text{st}}$, 2$^{\text{nd}}$ and 3$^{\text{rd}}$ NN exchange parameters from this work are $-1.7$ meV, 0 meV and $+4.0$ meV, respectively. The interlayer exchange value used in both sets of calculations is $+7.0$ meV. Both sets of calculations yield qualitatively similar results, with small differences in the Néel temperature and coercive magnetic fields.

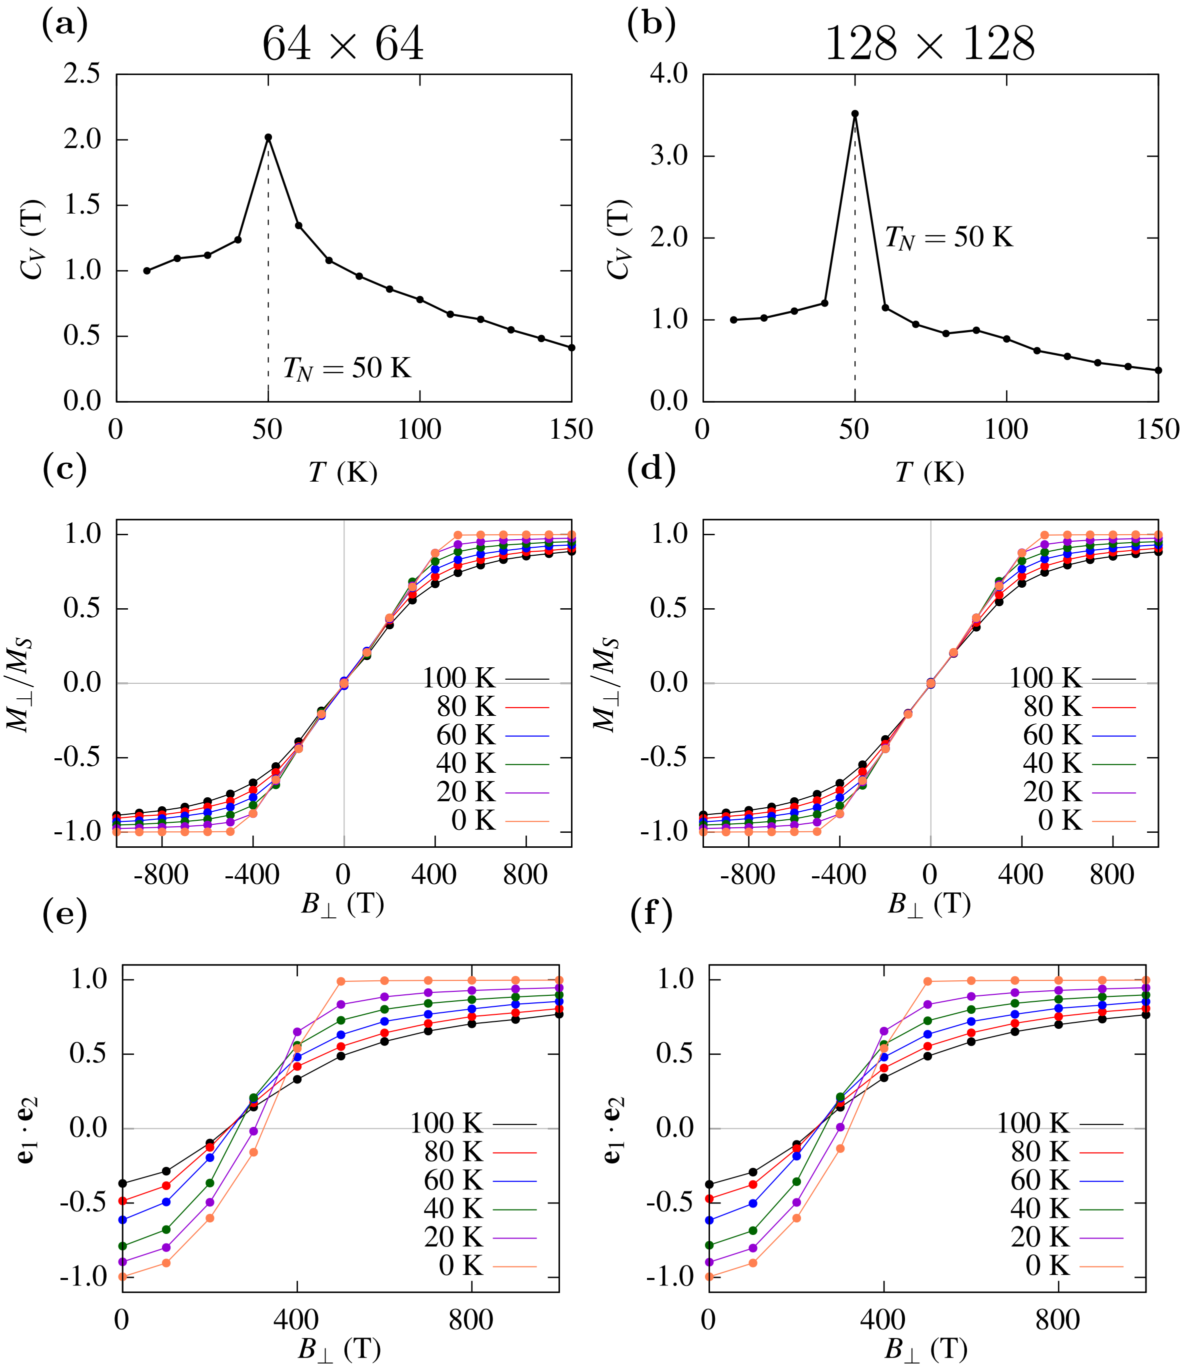


FIG. S9. **(a)**–**(b)** Specific heat $C_V$ of the system as a function of temperature $T$ from MC simulations for **(a)** a $64 \times 64$ supercell and **(b)** a $128 \times 128$ supercell. $C_V$ is normalized such that $C_V(T \to 0) = 1$. **(c)**–**(d)** Magnetic moment as a function of perpendicular magnetic field $B_\perp$ and temperature, for **(c)** a $64 \times 64$ supercell and and **(d)** a $128 \times 128$ supercell. **(e)**–**(f)** Relative alignment between the spins in each layer, $\mathbf{e}_1 \cdot \mathbf{e}_2$ as a function of perpendicular magnetic field $B_\perp$ and temperature, for **(e)** a $64 \times 64$ supercell and **(f)** a $128 \times 128$ supercell.

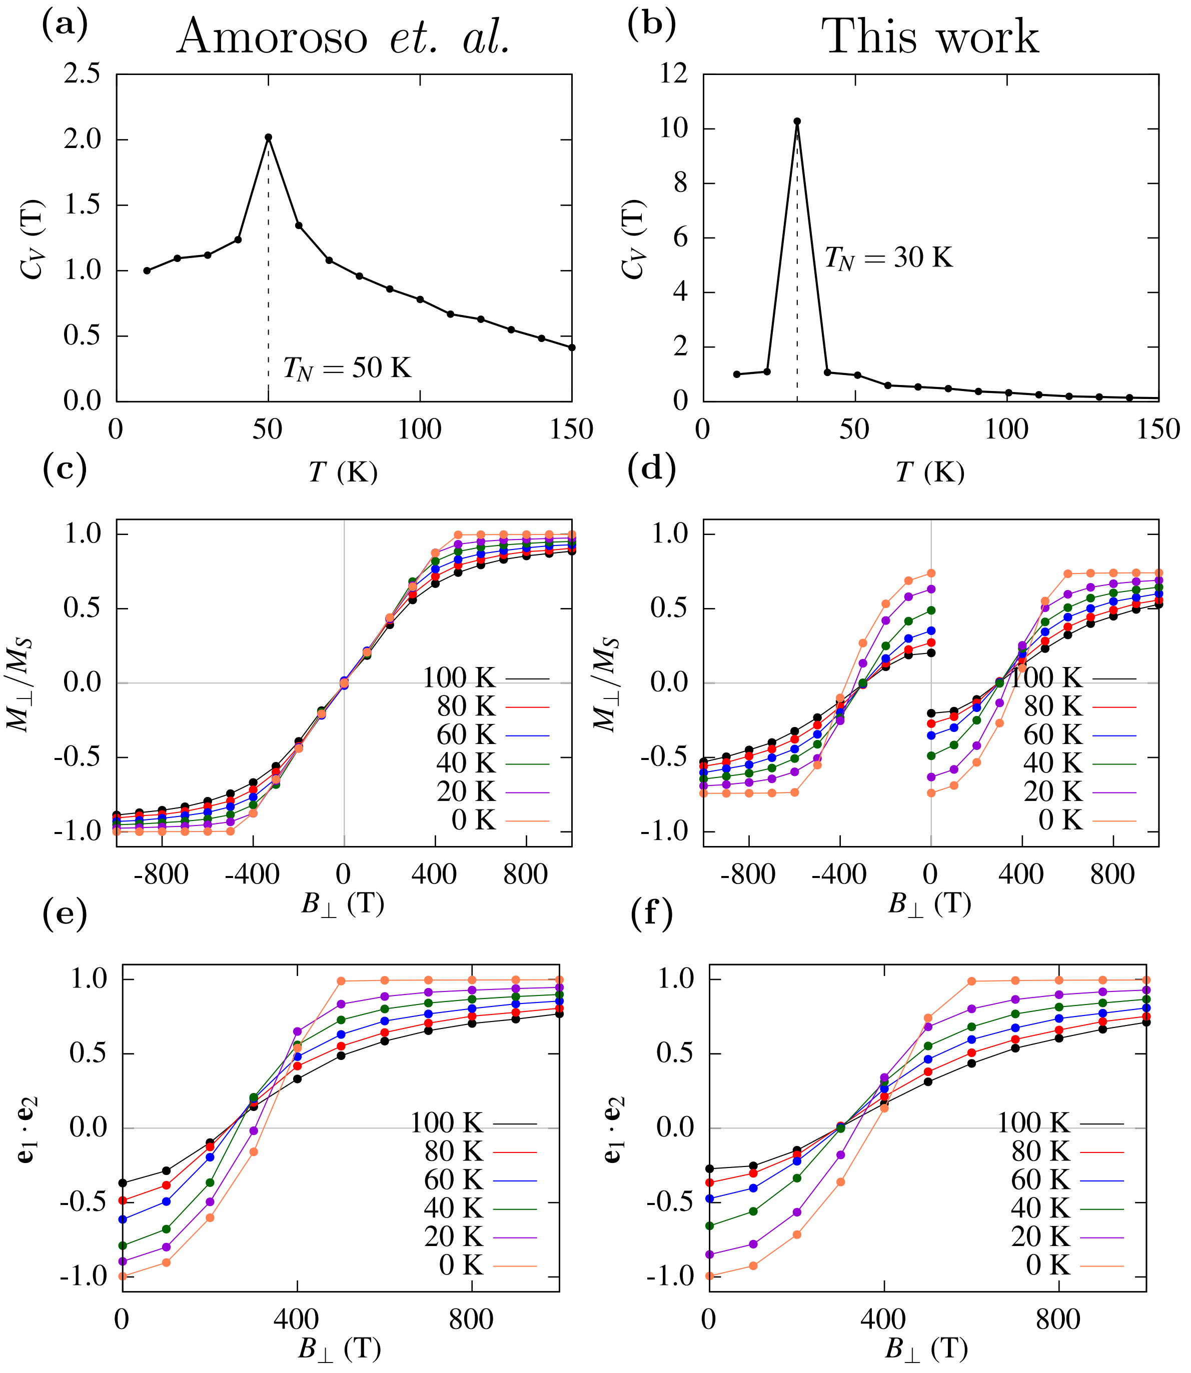


FIG. S10. **(a)**–**(b)** Specific heat $C_V$ of the system as a function of temperature $T$ from MC simulations for **(a)** Ref. [11] and **(b)** this work. $C_V$ is normalized such that $C_V(T \to 0) = 1$. **(c)**–**(d)** Magnetic moment as a function of perpendicular magnetic field $B_\perp$ and temperature, for **(c)** Ref. [11] and **(d)** this work. **(e)**–**(f)** Relative alignment between the spins in each layer, $\mathbf{e}_1 \cdot \mathbf{e}_2$ as a function of perpendicular magnetic field $B_\perp$ and temperature, for **(e)** Ref. [11] and **(f)** this work.

## COMPARISON WITH OTHER VAN DER WAALS FERROELECTRICS

The stacking-dependent out-of-plane dipole moment of anti-aligned bilayer $NiI_2$ is compared with other vdW ferroelectrics in Fig. S11, namely rhombohedral bilayer hBN and $WSe_2$. The dipole moment in $NiI_2$ is comparable or larger than those of hBN and $WSe_2$, depending on the interlayer spin configuration.

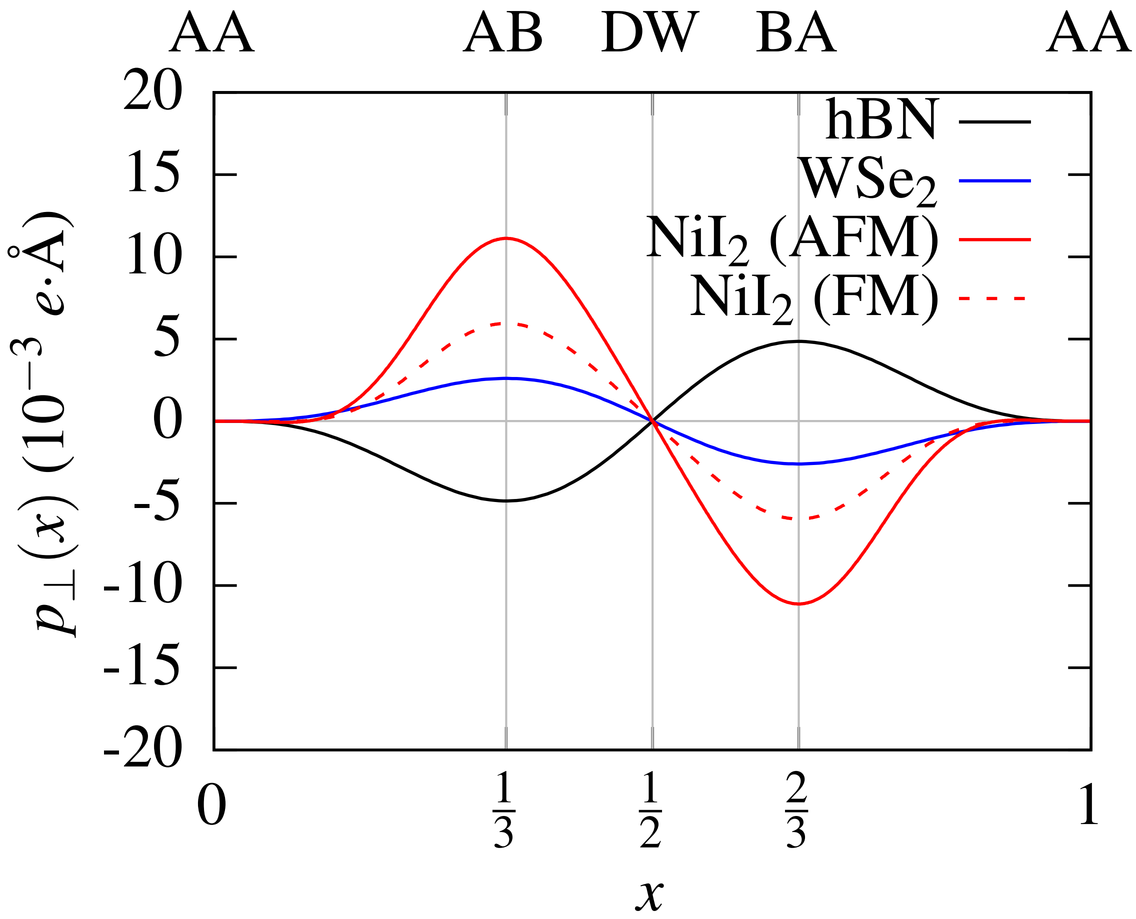


FIG. S11. Plot of the out-of-plane dipole moment as a function of stacking in bilayer hBN (black), $WSe_2$ (blue) and $NiI_2$ (red), for AFM (solid) and FM (dashed) interlayer spin configurations.

[1] J. M. Soler, E. Artacho, J. D. Gale, A. García, J. Junquera, P. Ordejón, and D. Sánchez-Portal, J. Phys. Condens. Matter **14**, 2745 (2002).
[2] D. Hamann, Phys. Rev. B **88**, 085117 (2013).
[3] A. García, M. J. Verstraete, Y. Pouillon, and J. Junquera, Comput. Phys. Commun. **227**, 51 (2018).
[4] M. Van Setten, M. Giantomassi, E. Bousquet, M. J. Verstraete, D. R. Hamann, X. Gonze, and G.-M. Rignanese, Comput. Phys. Commun. **226**, 39 (2018).
[5] N. R. Papior, G. Calogero, and M. Brandbyge, J. Phys.: Condens. Matter **30**, 25LT01 (2018).
[6] X. Gonze, B. Amadon, P.-M. Anglade, J.-M. Beuken, F. Bottin, P. Boulanger, F. Bruneval, D. Caliste, R. Caracas, M. Côté, *et al.*, Comput. Phys. Commun. **180**, 2582 (2009).
[7] H. J. Monkhorst and J. D. Pack, Phys. Rev. B **13**, 5188 (1976).
[8] J. P. Perdew, K. Burke, and M. Ernzerhof, Phys. Rev. Lett. **77**, 3865 (1996).
[9] S. Grimme, J. Antony, S. Ehrlich, and H. Krieg, J. Chem. Phys. **132** (2010).
[10] J. Neugebauer and M. Scheffler, Phys. Rev. B **46**, 16067 (1992).
[11] D. Amoroso, P. Barone, and S. Picozzi, Nat. Commun. **11**, 5784 (2020).
[12] M. J. Rutter, Comput. Phys. Commun. **225**, 174 (2018).
[13] D. Bennett, G. Chaudhary, R.-J. Slager, E. Bousquet, and P. Ghosez, Nat. Commun. **14**, 1629 (2023).
[14] G. Martínez-Carracedo, L. Oroszlány, A. García-Fuente, B. Nyári, L. Udvardi, L. Szunyogh, and J. Ferrer, Phys. Rev. B **108**, 214418 (2023).
[15] A. I. Liechtenstein, M. Katsnelson, V. Antropov, and V. Gubanov, J. Magn. Magn. Mater. **67**, 65 (1987).
[16] N. Sivadas, S. Okamoto, X. Xu, C. J. Fennie, and D. Xiao, Nano Lett. **18**, 7658 (2018).
